# Supplementary material for: Blue phosphorene bilayer is a two-dimensional metal -- and an unambiguous classification scheme for buckled hexagonal bilayers
Source: arXiv:2007.11027 source file (2020-09-14)
Supplement: Supplementary file 1 [file SM.pdf]

# Supplementary Material

# Blue phosphorene bilayer is a two-dimensional metal - and an unambiguous classification scheme for buckled hexagonal bilayers

Jessica Arcudia,[1] Roman Kempt,[2] Miguel E. Cifuentes-Quintal,[1] Thomas Heine,[2,3,4,*] and Gabriel Merino.[1,†]

[1]Departamento de Física Aplicada, Centro de Investigación y de Estudios Avanzados, Unidad Mérida, Mérida, Yucatán, México.

[2]Technische Universität Dresden, Fakultät für Chemie und Lebensmittelchemie, Bergstraße 66c, 01062 Dresden, Germany

[3]Helmholtz Zentrum Dresden-Rossendorf, Leipzig Research Branch, Permoserstr. 15, 04318 Leipzig, Germany

[4]Department of Chemistry, Yonsei University, Seodaemun-gu, Seoul 120-749, Republic of Korea

thomas.heine@tu-dresden.de

gmerino@cinvestav.mx

**Table S1.** The relative energies (*ΔE*) in meV/atom for all hexagonal bluP and grAs stacking configurations, computed at the PBE+MBD, PBE0+MBD and RPA+rSE@PBE levels including ZPE correction. Units are in meV/atom.

| | bluP BL | | | grAs BL | | |
|---|---|---|---|---|---|---|
| **System** | **PBE+ MBD** | **PBE0+ MBD** | **RPA+rSE@ PBE** | **PBE+ MBD** | **PBE0+ MBD** | **RPA+rSE@ PBE** |
| $A_1B_{-1}$ | 0.0 | 11.4 | 0.0 | 1.9 | 4.7 | 0.0 |
| $A_1A_1$ | 21.3 | 0.0 | 77.1 | 2.4 | 0.0 | 25.7 |
| $A_1B_1$ | 22.2 | 1.4 | 80.1 | 0.0 | 0.1 | 16.1 |
| 2-$A_1B_{-1}$ | 25.5 | 4.7 | 99.0 | - | - | - |
| $A_{-1}B_1$ | 30.1 | 10.4 | 123.1 | 16.7 | 15.3 | 108.9 |
| $A_1A_{-1}$ | 30.5 | 10.9 | 125.4 | 17.8 | 16.2 | 96.5 |

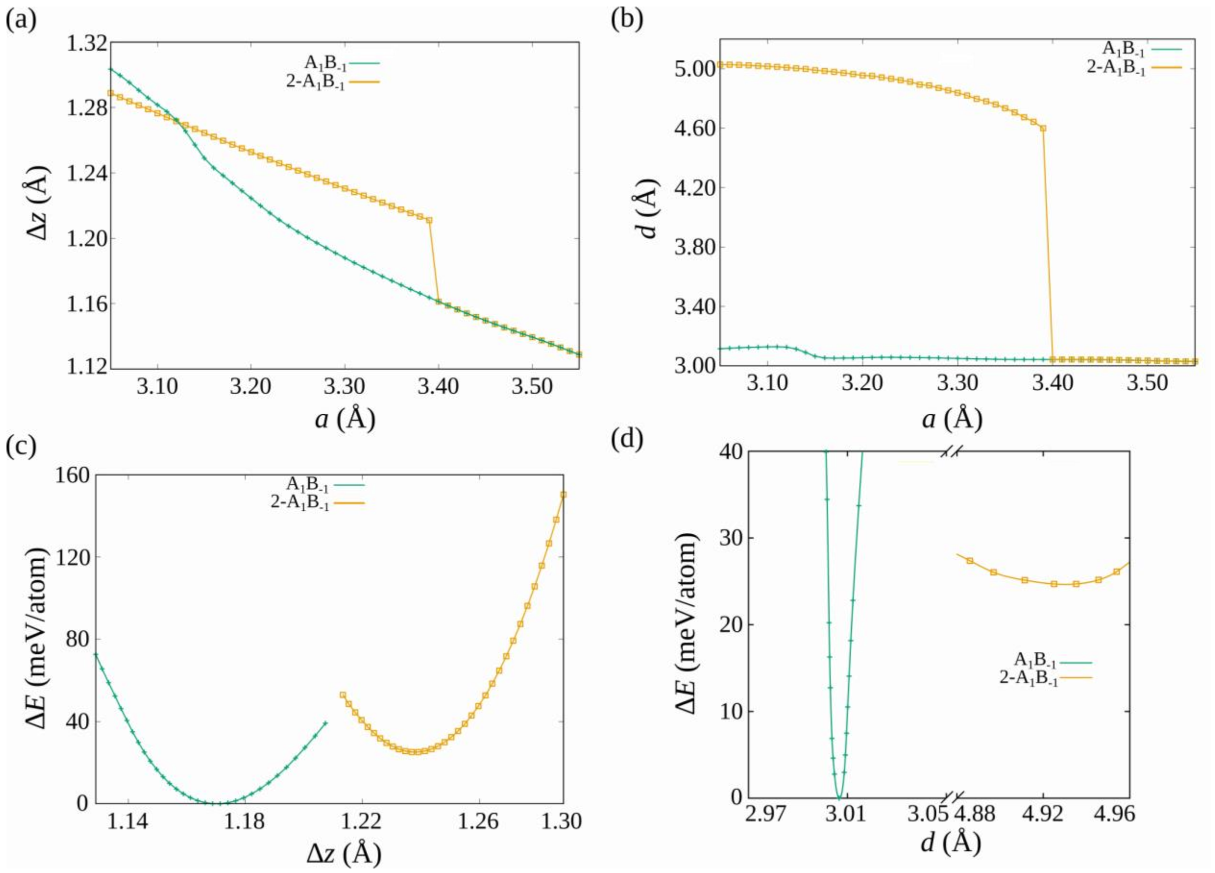


**Figure S1.** Variation of the (a) buckling, $\Delta z$, and (b) interlayer distance, $d$, with respect to the lattice constant, $a$, for the structure with two minima, $A_1B_{-1}$. Total energy, in meV/atom as a function of (c) $\Delta z$, and (d) $d$.

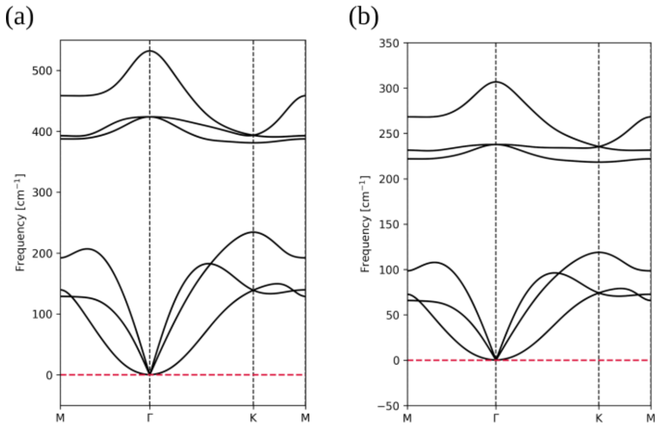


**Figure S2**. Phonon bands of hexagonal monolayers: (a) phosphorene, and (b) arsenene.

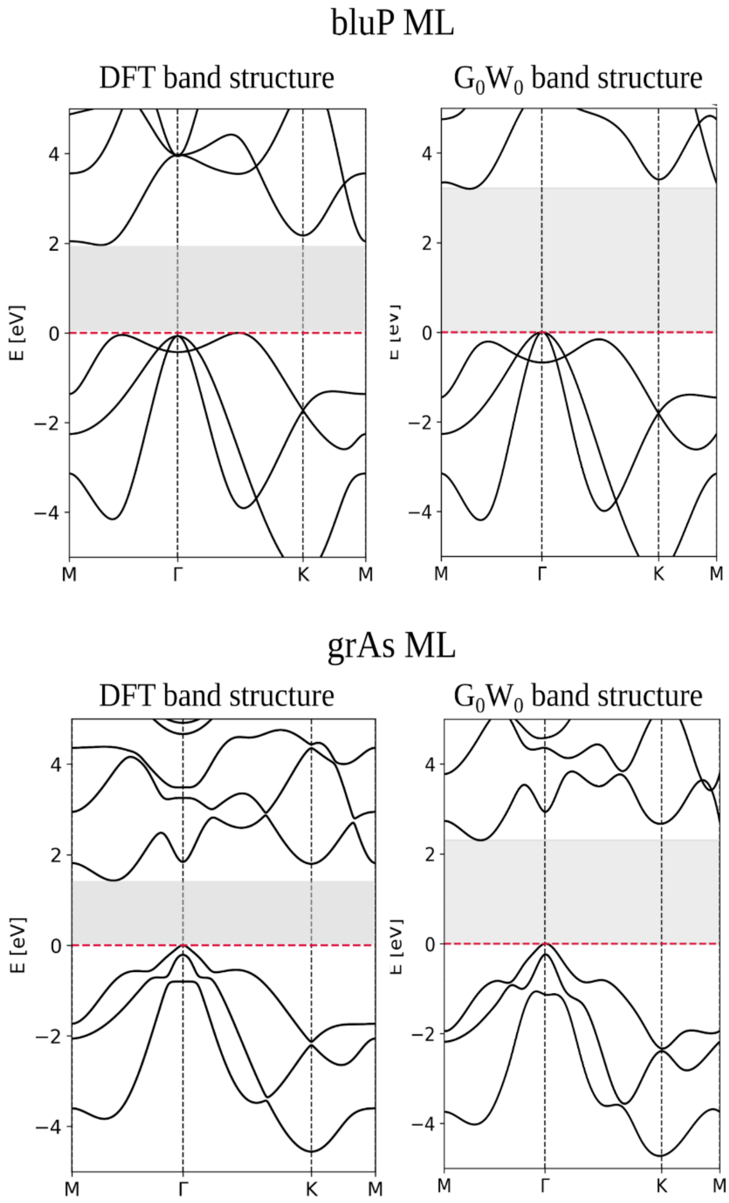


**Figure S3.** DFT and $G_0W_0$ electronic band structures of bluP and grAs ML.
